# Supplementary material for: Adapting Pre-trained Language Models for Quantum Natural Language Processing
Source: arXiv:2302.13812 source file (2023-02-24)
Supplement: Supplementary file 1 [file appendix.tex]

\section{Background Definitions}\label{sec:app_background}

\subsection{Complex Numbers and Complex Operations}
\label{sec:complex}

\begin{figure}[hb!] 
\centering 
\includegraphics[width=0.48\textwidth]{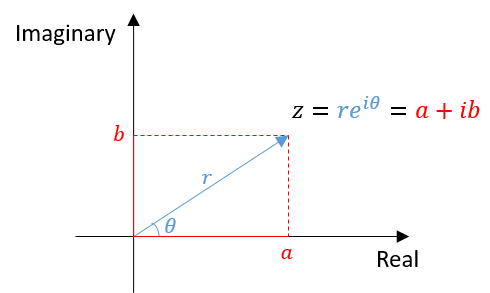}
\caption{Complex number in Cartesian and polar plane.} 
\label{fig:Rotate}
\end{figure}

A complex number $z$ is an ordered pair of real numbers. In the \textit{rectangular form}, it can be expressed as $z = (a,b)$ or $z =a+bi$ where $a$ and $b$ are the \emph{real} and \emph{imaginary} parts, respectively, and $i = \sqrt{-1}$. In the \textit{polar form}, $z$ can be expressed as $z= re^{i\theta} = r(\cos \theta + i\sin \theta)$,  where $r \in [0, +\infty)$ and $\theta \in [-\pi, \pi)$ are the \textit{modulus} and \textit{argument} (or \textit{amplitude} and \textit{phase}), resp.. We denote $\mathfrak{Re}$(z) and $\mathfrak{Im}$(z) as the real and imaginary parts of the complex number $z$, and as $|z|$ and $\mathfrak{arg}$(z) its modulus and argument. Fig.~\ref{fig:Rotate} plots both forms of a complex number.

%\noindent \textbf{Conjugate}. 
The \textbf{conjugate} of a complex number $z = a+bi$ is $\overline{z} = a-bi$.  In the polar form, the conjugate of $z = re^{i\theta}$ is $\overline{z} = re^{-i\theta}$. The inner product of two complex vectors $\bm{a}=[a_1,...,a_n]$ and $\bm{b}=[b_1,...,b_n]$ is the \textit{Hermitian inner product}, i.e. $\langle \bm{a}, \bm{b}\rangle = \bm{a}\bm{b}^H = \sum_{i=1}^n a_i\overline{b_i}$. Hence, the squared l2-norm of a complex vector $\bm{a}$ is $\bm{|a|} = \langle \bm{a}, \bm{a}\rangle = \sum_{i=1}^n a_i\overline{a_i} = \sum_{i=1}^n |a_i|^2$, and a pair of orthogonal vectors $\bm{a}, \bm{b}$ satisfy $\langle \bm{a}, \bm{b}\rangle = \bm{a}\bm{b}^H = \sum_{i=1}^n a_i\overline{b_i} = 0$. 

For matrices, the \textit{Hermitian transpose} is the conjugate transpose of a complex matrix $A$, denoted as $A^H = \overline{A^T}$. A \textit{semi-orthogonal} or \textit{semi-unitary} matrix $U \in \mathbb{C}^{m\times n}$ has mutually orthogonal columns when $m>n$, and $A^HA = I_n$. When $m=n$, $U$ is \textit{orthogonal} or \textit{unitary} with mutually orthogonal columns and rows. Both the columns and rows form an orthogonal basis of the space $\mathbb{C}^n$. 

The \textbf{mean and variance} of a set of complex numbers $\{z_j\}_{j=1}^n$ are given below:

\begin{equation}
\label{eq:stats}
    \begin{aligned}
        \bar{\textbf{z}} &= \frac{\sum_{j=1}^n {z_i}}{n} \\ \nonumber
        \sigma^2_z &= \frac{\sum_{j=1}^n {(z_j-\bar{\textbf{z}})(\overline{z_j-\bar{\textbf{z}}})}}{n}.
    \end{aligned}
\end{equation}

\subsection{Classical BERT}
\label{sec:bert}

Multi-layer transformer~\citep{vaswani_attention_17} is the backbone architecture of BERT. A transformer layer has a multi-head scaled dot-product attention module at its core:

\begin{equation}
\resizebox{0.48\textwidth}{!}{
    $
    \begin{aligned}
    \text{MultiHead}(Q,K,V) = \text{Concat}(\text{head}_1,...,\text{head}_h)W^O \\ \nonumber
     \text{head}_i = \text{Attention}(QW_i^Q,KW_i^K, VW_i^V)W_i^O.
     \end{aligned}
     $
     }
\end{equation}

$\{W_i^Q, W_i^K, W_i^V, W_i^O\}$ are linear projection matrices, and $Q=K=V=H$ is the packed hidden representations of all elements in the previous transformer layer. The attention function is a softmax-normalized pairwise scaled dot-product for each pair of elements in the sequence:

\begin{equation}
    \text{Attention}(Q,K,V) = \text{softmax}(\frac{QK^T}{\sqrt{d_k}})V.
\end{equation}

The output of the attention module is passed to a point-wise feed-forward network to produce the final output of the transformer layer.

BERT starts with an embedding layer that adds positional embedding, token embedding and segment embedding of the concatenated segments. The embeddings are fed into a stack of $N$ transformer layers. The last hidden units of each sequence are used to perform Mask Language Model (MLM) and Next Sentence Prediction (NSP). The MLM objective $\mathcal{L}_{MLM}$ is a cross-entropy loss on predicting the masked tokens. BERT randomly selects 15\% of the input tokens for possible replacement. Of the selected tokens, 80\% are replaced with [MASK], 10\% are left unchanged, and 10\% are replaced by a randomly selected vocabulary token. NSP is a binary classification task for predicting whether the two segments follow each other in the original text. Positive and Negative inputs are sampled from consecutive sentences and nonconsecutive sentences with equal probability. The binary cross-entropy loss $\mathcal{L}_{NSP}$ is added with the MLM objective to the overall objective of BERT: $\mathcal{L}_{BERT} = \mathcal{L}_{MLM}+ \mathcal{L}_{NSP}$. 

The BERT model is pre-trained on large volumes of text corpora, e.g. BOOKCORPUS and the English WIKIPEDIA~\citep{devlin2019bert}. The model is further fine-tuned on different text classification and natural language inference (NLI) datasets, such as the famous GLUE benchmark~\citep{wang2019glue}. The average effectiveness values over all datasets, called GLUE score, is taken as the indicator of its performance.

\section{Missing details in the description of model components}\label{app:s:comp}

\subsection{Rationale behind complex-valued word embeddings}
\label{sec:rationale_cpe}

The polar form of complex value has been found to be a feasible way of encoding different levels of information in word embeddings~\citep{li2019cnm,wang2019semantic,Li2018Quantum}. The idea is to draw an analogy between word positions and wave functions, and encode word positions to phases of a complex embedding scheme, compatible with the transformer architecture \citet{Wang2020encoding}. 

The proposed embedding scheme makes sense in theory. The token embedding impacts the most word semantics as it determines the amplitudes of the embedding. The frequency and initial phase embeddings influence word semantics less, but are needed to determine the interactions between words in the attention mechanism. The segment embedding plays a lesser role in the token semantics. 

\noindent \textbf{Complex-valued embedding with shared frequencies.} Shared frequency embeddings have been recommended by~\citet{Wang2020encoding} as a parameter-saving and effective complex embedding scheme. This setting inspired ~\citet{su2021roformer} to enhance the transformer with \textit{rotary position embeddings} (ROPE). In its mathematical form, ROPE is a real-valued version of the frequency-shared embedding with mapping $\mathcal{P}: \mathbb{Z}^D \rightarrow \mathbb{R}^{2d}$ that maps $\textbf{z} =[x_1+ix_2, x_3+ix_4,...,x_{2D-1}+ix_{2D}]$ to $\textbf{x} =[x_1, x_2,...,x_{2D}]$ for all vectors involved. The chosen frequency embedding values led to strong performance on sequence to sequence (seq2seq) tasks. In this work, we study whether shared frequency embeddings can also benefit a pre-trained LM. As per~\citet{su2021roformer}, we fix the shared frequency $w_j = w = \{ 10000^{-(i-1)/D}, i \in [1,2,...,D]\} \in \mathbb{R}^D$, and set the remaining embeddings $\{R, S, \Theta\}$ trainable.

\subsection{Complex multi-head attention}\label{sec:app_mha}

The formula for one attention head is given by

\begin{equation}
    \text{ComplexAttention}(Q,K,V) = f(\frac{QK^H}{\sqrt{d_k}})V.
\end{equation}

where $f(\cdot)$ is a softmax-like activation function. We need to extend the real softmax function to the complex domain to handle complex-valued inputs.

A straightforward approach to this aim is to apply softmax to real and imaginary parts of the inner product separately. Suppose the Hermitian product is denoted by $\{\sigma(q,k)\}$ for a pair of query-key elements $(q,k)$, the formula of this \textit{split activation function} is given by

\begin{equation}\label{eq:app_split_softmax}
     f_\text{split}(q,k) = \frac{e^{\mathfrak{Re}(\sigma(q,k))}}{\sum_{k'}{e^{\mathfrak{Re}(\sigma(q,k'))}}} +i \frac{e^{\mathfrak{Im}(\sigma(q,k))}}{\sum_{k'}{e^{\mathfrak{Im}(\sigma(q,k'))}}},
\end{equation}

where the summation iterates over all key elements $k'$ in the sequence. The split softmax function normalizes  both real and imaginary parts of the affinity scores to sum up to 1 for each key. When the scores are taken to linearly combine the value vectors $\{v'\}$, the summation can be decomposed into

\begin{equation}
    \resizebox{0.48\textwidth}{!}{
    $
        \begin{aligned}
         h &= \sum_{k'} f(q,k')v' \nonumber \\
         &= \sum_{k'} (\mathfrak{Re}(f(q,k'))\mathfrak{Re}(v')-\mathfrak{Im}(f(q,k'))\mathfrak{Im}(v')) \nonumber \\
          &+i\sum_{k'} (\mathfrak{Re}(f(q,k'))\mathfrak{Im}(v')+\mathfrak{Re}(f(q,k'))\mathfrak{Im}(v')),
        \end{aligned} 
    $
    }
\end{equation}

\noindent and a negative sign exists in the real part of the summation due to the fact that $i^2 = -1$. On the contrary, an ideal weighted combination should be a convex combination of the value vectors with all non-negative weights. This motivates us to design normalization functions $f$ that produce real-valued affinity scores from the complex inputs, because they indicate a convex combination in both the real and imaginary channels. Two more natural choices are to apply softmax normalization to the amplitude and real part of the complex numbers, as shown in the equations below\footnote{taking the imaginary part for softmax normalization is equivalent to taking the real part.}.

\begin{equation}\label{eq:app_mod_softmax}
     f_\text{amp}(q,k) =\frac{e^{|\sigma(q,k)|}}{\sum_{k'}{e^{|\sigma(q,k')|}}}
\end{equation}

\begin{equation}\label{eq:app_real_softmax}
  f_\text{re}(q,k) = \frac{e^{\mathfrak{Re}(\sigma(q,k))}}{\sum_{k'}{e^{\mathfrak{Re}(\sigma(q,k'))}}}.
\end{equation} \\

\noindent In a previous work,~\citet{yang2018glomo} replaced softmax with a squared ReLU function to compute the attention scores between nodes of a graph. The formula is 

\begin{equation}
     f_\text{sq-ReLU}(q,k) = \frac{(\text{ReLU}(\sigma(q,k)+b))^2}{\sum_{k'}{(\text{ReLU}(\sigma(q,k')+b))^2}}, 
\end{equation}

where $b$ is a real bias scalar. As demonstrated in~\citep{yang2018glomo}, the introduction of ReLU effectively enforces sparsity and the use of square operations stabilizes training for graph neural networks. Inspired by the empirical superiority, we propose a similar activation function that converts complex affinity scores to real attention scores. The mathematical expression is given by

\begin{equation}\label{eq:normedzrelu}
     f_\text{sq-zReLU}(q,k) = \frac{|\text{zReLU}(\sigma(q,k)+b)|^2}{\sum_{k'}{|\text{zReLU}(\sigma(q,k')+b)|^2}}, 
\end{equation}
    
where zReLU is a complex version of ReLU, and $b$ is a complex-valued scalar bias. A typical implementation of zReLU is given by
\begin{equation}~\label{eq:zrelu}
    \text{zReLU}(z)= \left\{\begin{array}{ll}
    z &  \mathfrak{Re}(z), \mathfrak{Im}(z) \geq 0 \\
    0 &  \text{otherwise} \\
    \end{array} 
    \right .
\end{equation}

which masks out complex values with a negative real or imaginary part. Since zReLU produces a complex-valued output, we take its squared amplitudes to avoid the presence of negative terms in the weighted linear summation of value vectors.

\subsection{Complex activation function}~\label{sec:app_activation}
We consider ReLU and GeLU variants for the design of complex-valued activation functions. The most intuitive extension is to apply ReLU and GeLU to the real and imaginary parts respectively. This guarantees that all complex values have non-negative real and imaginary parts after activation. Suppose the input values are centered at zero, the split activation function is expected to drops 50\% information, which is the same as the real-valued case. However, many complex values are partly activated by this function with real or imaginary parts masked. Therefore, we seek to design alternative functions that always activate pr mask a complex value as a whole.  The following variants are taken into consideration:

\begin{itemize}
    \item {\textbf{zReLU}. We zero out complex numbers with non-positive real or imaginary parts and only keep the ones with non-negative values on both components. 75\% percent values are expected to the dropped by this function. Adopted in a previous complex-valued deep neural network~\citep{trabelsi2018deep}.
    }
    
   \item{\textbf{argReLU}. Another strategy is to consider the polar form of complex numbers and filter out values within a certain argument. Essentially, the formula reads
   \begin{equation} \label{eq:angular-zrelu}
        z_{out} = \left\{\begin{array}{ll} 
      z & arg(z) \in [\theta_1, \theta_2] \\
      0 & \text{otherwise}\\
        \end{array} 
        \right .
    \end{equation}
    By choosing a proper interval $\theta_1, \theta_2 \in [-\pi,\pi]$, one can control the ratio of masked parameters. Note that argReLU is a generalization of the above-mentioned zReLU function, which corresponds to $\theta_1=0, \theta_2=\frac{\pi}{2}$. It was first introduced in~\citep{guberman2016complex}.
    }
    
    \item {\textbf{modReLU}.  Under the polar form, we can also apply activation onto the modulus of a complex number. Since the modulus is always non-negative, we apply a negative bias term to the amplitude before passing it to an ReLU function:
    \begin{equation}\label{eq:modrelu}
        z_{out} = \left\{\begin{array}{ll} 
      \frac{|z|+b}{|z|} z & |z|+b \geq 0 \\
      0 & \text{otherwise} \\
        \end{array} 
        \right .
    \end{equation}
    where $b$ is a negative real bias term. It was previously adopted in complex-valued neural networks~\citep{trabelsi2018deep}.
    }
    \item {\textbf{modGeLU}.  GeLU essentially computes the Gaussian cumulative distribution function as a non-linear weight applied to the input, i.e. $y=xP(X\leq x)$. Instead of activating the real and imaginary channels based on their respective distribution function, we may compute the cumulative distribution function of the modulus as a weight for activating the whole complex value, i.e. $z_{out} = zP(|Z|\leq |z|)$. Following the implementation of GeLU in Google BERT repository, the formula is
    \begin{equation}\label{eq:modgelu}
        \resizebox{0.44\textwidth}{!}{
        $
        z_{out} = 0.5 z (1 + tanh(\sqrt{\frac{2}{\pi}}(|z|+0.044715|z|^3)) \nonumber \\ 
        $
        }
    \end{equation}
    }
\end{itemize}

% \subsubsection{Complex fully-connected layer}\label{sec:app_dense}
% The implementation of a complex fully-connected layer is introduced in Section~\ref{sec:complex}, following Eq.~\ref{eq:complex_dense}. In particular, for an input vector $\bm{X} \in \mathbb{C}^{d_i}$, a fully-connected layer projects it to a $d_o$-dim vector $z \in \mathbb{C}^{d_o}$, with weight matrix $\bm{W} \in \mathbb{C}^{d_o \times d_i}$ and a bias term $\bm{b} \in \mathbb{C}^{d_o}$.

% The orthogonality of neural network weights has been widely studied in previous works~\citep{wang2020orthogonal, singla2021skew, trockman2021orthogonalizing, trabelsi2018deep, wisdom2016full, arjovsky2016unitary}. Most of them directly enforce the weight matrix to be orthogonal during the training procedure, leading to a high stability~\citep{wisdom2016full, arjovsky2016unitary} and robustness~\citep{wang2020orthogonal, singla2021skew, trockman2021orthogonalizing}, at little cost in accuracy performance. In addition, introducing orthogonality as a regularization term~\citep{zhang-etal-2021-orthogonality} or performing orthogonal initialization~\citep{trabelsi2018deep} of network weights can also boost model performance. Due to its incurred computational cost, enforcing the orthogonality constraint on network weights is not leveraged in our study. We study the impact of orthogonal regularization on transformer attention scores and dense weights in Section~\ref{sec:app_reg}, and examine the effect of orthogonal weight initialization in Section~\ref{sec:app_weight_init}.

\subsection{Complex dropout layer}\label{sec:app_dropout}

We implement the complex dropout layer by simply extending the real case. At a probability $p$, we randomly drop out complex values in a complex tensor. 

\subsection{Orthogonal regularization}\label{sec:app_reg}
In a recent study,~\citet{zhang-etal-2021-orthogonality} discovered that imposing orthogonality constraints on attention scores and dense weights can boost the empirical performance of a multi-layer transformer model. We are hence motivated to study the effect of orthogonality constraints for our model, which has a deeper architecture with complex-valued weights, and trained on a significantly larger volume of data. \\

\noindent \textbf{Orthogonality constraints on attention scores.} We impose constraints on the affinity matrix $A$, whose rows are the post-activation attention scores for each key:
\begin{equation}
    A = softmax(\frac{QK^T}{\sqrt{d_k}})
\end{equation}

~\citet{zhang-etal-2021-orthogonality} argues that the affinity matrix is robust to query perturbations when its rows are independent of each other. Inspired by this merit, we propose the loss term below to punish the dependence of different rows:

\begin{equation}\label{eq:att-ortho-reg}
    \mathcal{L}_{AR} = \lambda ||AA^H-diag(AA^H)||^2_F,
\end{equation}

where $diag(A)$ stands for taking the diagonal elements of the matrix A only, and $F$ stands for matrix Frobenius norm. The inner product of each pair of rows of A corresponds to an off-diagonal entry in $AA^H$, so we compute the sum of their squared values to regularize the independence of A rows. We take the off-diagonal entries by subtracting the matrix $AA^H$ by its diagonal elements. In contrast, ~\citet{zhang-etal-2021-orthogonality} proposes the term below:
\begin{equation}\label{eq:dense-ortho-reg}
    \hat{\mathcal{L}}_{AR} = \lambda ||AA^T-I||^2_F.
\end{equation}

Since $A$ is the post-softmax score matrix, its rows are always sum to 1 each.  $\hat{\mathcal{L}}_{AM}$ constrains each row to be not only mutually orthogonal \textit{but unit in length}, which simply means a one-hot vector under the unit-sum condition\footnote{if $\sum {a_i}= \sum {a_i}^2 =1$ for non-negative real values ${a_i}$, ${a_i}$ must have a single 1 and the remaining values are all zeros.}. In this way, $A$ is driven to a permutation matrix, which is undesired for attention scores. In contrast, we relaxed the unit length constraint in the revised loss term, so that the only constraint is placed on the mutual independence of attention scores for different keys.\\

\noindent \textbf{Orthogonality constraints on dense weights.}  The motivation behind this setting is that when the weights in fully-connected weights $W$ are orthogonal, the Lipschitz constant of the linear projection is no greater than one, which indicates numerical stability during training~\citep{zhang-etal-2021-orthogonality}. Therefore, we introduce the following loss term to constrain the orthogonality of weight matrices:

\begin{equation}\label{eq:both-ortho-reg}
    \mathcal{L}_{LR} = \lambda \sum_i||W_iW_i^H-I||^2_F,
\end{equation}

where the summation iterates over all complex-valued dense weights in the network. \\

\noindent \textbf{Combining the orthogonality constraints.} Our model computes an attention matrix at each transformer layer for each sample with \textit{the same weights}, so the affinity matrices has an extra dimension over the dense weights. When we combine both loss terms, they should be normalized to the same scale before added together. For a batch of $M$ samples, the affinity matrix regularization loss should be divided by $M$ before adding with the dense weight regularization loss. The overall regularization term $L_{OR}$ is computed as

\begin{equation}
    \begin{aligned}
       \mathcal{L}_{OR} &= \lambda (\sum_i||W_iW_i^H-I||^2_F \\ \nonumber
       &+ \frac{1}{M}\sum_j ||A_jA_j^H-tr(A_jA_j^H)||^2_F), \\
    \end{aligned}
\end{equation}

where the index $j$ iterates over the affinity matrices of all transformer layers for all samples in the batch. When taken into consideration, $\mathcal{L}_{AR}$, $\mathcal{L}_{LR}$ or $\mathcal{L}_{OR}$ is added to the original loss terms $\mathcal{L}_{NSP}$ and $\mathcal{L}_{MLM}$ as the final loss function of the network.

\section{Model settings}\label{sec:app_settings}

We have presented and discussed various settings for different model components. Below we summarize the included settings in our study. Table~\ref{tab:model_components} presents the individual components with pointers to sections in the main body or appendix that describe them. It also shows the per-component settings for each of the overall models.

\noindent \textbf{Embedding.}  By default, we adopt \textbf{split-embed}, which sums up the complex-valued token, position and segment embeddings. We also experiment with \textbf{general-complex-embed}, the general complex-valued embedding scheme given by Eq.~\ref{eq:complex_embedding}, as well as the frequency-shared scheme, named \textbf{rotary-embed} in that it adopts the fixed shared frequency values $w_j = w = \{ 10000^{-(i-1)/D}, i \in [1,2,...,D]\} \in \mathbb{R}^D$ in Rotary Transformer~\citep{su2021roformer}. 
Considering their non-negative nature, we randomly initialize token and segment embeddings from Rayleigh distributions with Glorot mode.\\

\noindent \textbf{Activation.} The default activation function for attention is \textbf{attn-split-softmax}, which applies softmax normalization to real and imaginary parts respectively. In addition, we implement softmax on the modulus and real part of the affinity scores following Eq.~\ref{eq:app_mod_softmax} and \ref{eq:app_real_softmax}. They are denoted by \textbf{attn-mod-softmax} and \textbf{attn-real-softmax} respectively. We also include \textbf{attn-squaredzrelu}, the activation function proposed in~\citet{yang2018glomo} and extended to the domain for the complex-valued scores.

For hidden units, we apply ReLU activation to the real and imaginary parts of hidden units respectively as the default setting, namely \textbf{hidden-split-relu}. The other types of activation functions in App.~\ref{sec:app_activation} are included and renamed as \textbf{hidden-zrelu}, \textbf{hidden-argrelu}, \textbf{hidden-modrelu} and \textbf{hidden-modgelu}. We also implement the split GeLU activation function \textbf{hidden-split-gelu} that separately performs GeLU to the real and imaginary components.\\

\noindent \textbf{Fully-connected Layer.}  We implement dense layers with complex-valued weights and bias. By default, we take the modulus of the last complex dense layer output for computing MLM and NSP loss. We also take into consideration the variants that take the real part of the dense output for computing training loss, and they are referred to as \textbf{mlm-real} and \textbf{nsp-real} respectively.\\

\noindent \textbf{Weight initialization.}  By default, we initialize the real and imaginary parts of complex weights with a normal distribution at a mean value of zero and a variance of 0.01, denoted by \textbf{split-init}. We also include unitary weight initialization (\textbf{unitary-init}) as well the phase-modulus strategies \textbf{rayleigh-he-init} and \textbf{rayleigh-glorot-init} as introduced in Sec.~\ref{sec:weight_init}.

\noindent \textbf{Normalization.} The default setting \textbf{split-layer-norm} takes the layer normalization onto real and imaginary parts respectively. In addition, we implement layer normalization to the real and imaginary parts respectively in the \textbf{complex-layer-norm} setting, whose formula is given in Eq.~\ref{eq:complex_layer_norm}.\\

\noindent \textbf{Regularization.} By default (\textbf{weight-decay}), we simply perform weigh decay in the complex AdamW optimizer, with no extra regularization terms added to the loss function. We also introduce orthogonality constraints on attention scores, dense weights and both of them as an additional loss term, in \textbf{att-ortho-reg}, \textbf{dense-ortho-reg} and \textbf{both-ortho-reg} respectively. The regularization coefficient $\lambda$ varies in $\{10^{-4},10^{-6},10^{-8},10^{-10}\}$. \\

\noindent \textbf{Optimization.}  We compare the complex-valued AdamW optimizer with the original AdamW optimizer for real numbers. The two optimizers are used to train the same model, which has all the default network settings. We refer to them as \textbf{cadam} and \textbf{radam} respectively.\\

\begin{landscape}
\begin{table}[!ht]
\caption{Model components, pointers to subsections that describe them, and adopted settings for each experimented \textbf{CVBERT} and \textbf{QBERT} model. }
\label{tab:model_components}
\begin{tabular}{c|l|c|c|c|c|c}
\hline
Component                                                                                  & Included Settings & \begin{tabular}[c]{@{}c@{}}CVBERT-default\\ (12L-768-3072)\end{tabular} & \multicolumn{1}{l|}{\begin{tabular}[c]{@{}l@{}}CVBERT-all-split\\ (CVBERT-default)\\ (12L-768-3072)\end{tabular}} & \multicolumn{1}{l|}{\begin{tabular}[c]{@{}l@{}}CVBERT-best-1\\ (12L-768-3072)\end{tabular}} & \multicolumn{1}{l|}{\begin{tabular}[c]{@{}l@{}}CVBERT-best-2\\(CVBERT-base)\\ (12L-768-1536)\end{tabular}} & \multicolumn{1}{l}{\begin{tabular}[c]{@{}l@{}}QBERT-base\\ (12L-768-1536)\end{tabular}} \\ \hline
\multirow{3}{*}{\begin{tabular}[c]{@{}c@{}}Embedding \\ (Sec.~\ref{sec:building_blocks}; App.~\ref{sec:rationale_cpe} )\end{tabular}} & \textbf{split-embed} & \textbf{\checkmark} & \textbf{\checkmark} & \textbf{\checkmark} & \textbf{\checkmark} & \textbf{\checkmark} \\ \cline{2-7} & \textbf{general-complex-embed} & \textbf{} & \textbf{} & \textbf{} & \textbf{} & \textbf{} \\ 
\cline{2-7} & \textbf{rotary-embed} & \textbf{} & \textbf{} & \textbf{} & \textbf{} & \textbf{} \\ \hline
\multirow{4}{*}{\begin{tabular}[c]{@{}c@{}}Multi-head attention\\ (Sec.~\ref{sec:building_blocks}; App.~\ref{sec:app_mha})\end{tabular}}  & \textbf{attn-split-softmax} & \textbf{\checkmark}  &  & \textbf{} & \textbf{} & \textbf{} \\ 
\cline{2-7} & \textbf{attn-real-softmax} & \textbf{} & \textbf{} & \textbf{} & \textbf{} & \textbf{} \\ 
\cline{2-7} & \textbf{attn-squaredzrelu} & \textbf{} & \textbf{} & \textbf{} & \textbf{} & \textbf{} \\ 
\cline{2-7} & \textbf{attn-modsoftmax} & \textbf{} & \textbf{\checkmark} & \textbf{\checkmark} & \textbf{\checkmark} & \textbf{\checkmark} \\ \hline
\multirow{6}{*}{\begin{tabular}[c]{@{}c@{}}Activation function\\ (Sec.~\ref{sec:activation}; App.~\ref{sec:app_activation})\end{tabular}} & \textbf{hidden-split-relu} & \textbf{\checkmark} &  & \textbf{} & \textbf{} & \textbf{} \\ 
\cline{2-7} & \textbf{hidden-argrelu} & \textbf{} & \textbf{} & \textbf{} & \textbf{} & \textbf{} \\ 
\cline{2-7} & \textbf{hidden-modrelu} & \textbf{} & \textbf{\checkmark} & \textbf{} & \textbf{} & \textbf{} \\ 
\cline{2-7} & \textbf{hidden-zrelu} & \textbf{} & \textbf{} & \textbf{} & \textbf{} & \textbf{} \\ 
\cline{2-7} & \textbf{hidden-split-gelu} & \textbf{} & \textbf{} & \textbf{\checkmark} & \textbf{\checkmark} & \textbf{\checkmark}\\ 
\cline{2-7} & \textbf{hidden-modgelu} & \textbf{} & \textbf{} & \textbf{} & \textbf{} & \textbf{}\\ \hline
\multirow{4}{*}{\begin{tabular}[c]{@{}c@{}}Fully-connected layer\\ (Sec.~\ref{sec:building_blocks})\end{tabular}} & \textbf{complex-dense} & \textbf{\checkmark} & \textbf{\checkmark} & \textbf{\checkmark} & \textbf{\checkmark} & \textbf{\checkmark}\\ 
\cline{2-7} & \textbf{mlm-real} & \textbf{} & \textbf{} & \textbf{} & \textbf{} & \textbf{} \\
\cline{2-7} & \textbf{mlm-modulus} & \textbf{\checkmark} & \textbf{\checkmark} & \textbf{\checkmark} & \textbf{\checkmark} & \textbf{\checkmark} \\
\cline{2-7} & \textbf{nsp-real} & \textbf{} & \textbf{} & \textbf{} & \textbf{} & \textbf{} \\
\cline{2-7} & \textbf{nsp-modulus} & \textbf{\checkmark} & \textbf{\checkmark} & \textbf{\checkmark} & \textbf{\checkmark} & \textbf{\checkmark} \\
\cline{2-7} & \textbf{nsp-measurement} & \textbf{} & \textbf{} & \textbf{} & \textbf{} & \textbf{\checkmark} \\ \hline
\multirow{4}{*}{\begin{tabular}[c]{@{}c@{}}Weight Initialization\\ (Sec.~\ref{sec:weight_init})\end{tabular}} & \textbf{split-init} & \textbf{\checkmark} & & \textbf{\checkmark} & \textbf{\checkmark} & \textbf{\checkmark} \\ 
\cline{2-7} & \textbf{rayleigh-he-init} & \textbf{} & \textbf{} & \textbf{} & \textbf{} &\textbf{}\\ 
\cline{2-7} & \textbf{rayleigh-glorot-init}  & \textbf{} & \textbf{\checkmark} & \textbf{} & \textbf{} & \textbf{}\\ 
\cline{2-7} & \textbf{unitary-init} & \textbf{} & \textbf{} & \textbf{} & \textbf{} & \textbf{} \\ \hline
\multirow{4}{*}{\begin{tabular}[c]{@{}c@{}}Normalization\\ (Sec.~\ref{sec:normalization})\end{tabular}} & \textbf{split-layer-norm} & \textbf{\checkmark} & & \textbf{} & \textbf{} & \textbf{} \\ 
\cline{2-7} & \textbf{complex-layer-norm} & \textbf{} & \textbf{\checkmark} & \textbf{\checkmark} & \textbf{\checkmark} & \textbf{} \\ 
\cline{2-7} & \textbf{mixed-layer-norm} & \textbf{} & \textbf{} & \textbf{} & \textbf{} & \textbf{\checkmark} \\ 
\cline{2-7} & \textbf{unit-norm} & \textbf{} & \textbf{} & \textbf{} & \textbf{} & \textbf{} \\ \hline
\multirow{4}{*}{\begin{tabular}[c]{@{}c@{}}Regularization\\ (Sec.~\ref{sec:reg}; App.~\ref{sec:app_reg})\end{tabular}} & \textbf{no-reg} & \textbf{\checkmark} & \textbf{\checkmark} & \textbf{\checkmark} & \textbf{\checkmark} & \textbf{\checkmark}\\ \cline{2-7} & \textbf{att-reg} & \textbf{} & \textbf{} & \textbf{} & \textbf{} & \textbf{}\\ \cline{2-7} & \textbf{hidden-reg} & \textbf{} & \textbf{} & \textbf{} & \textbf{} & \textbf{}\\ \cline{2-7} & \textbf{both-reg} & \textbf{} & \textbf{} & \textbf{} & \textbf{} & \textbf{} \\\hline
\multirow{2}{*}{\begin{tabular}[c]{@{}c@{}}Optimization\\ (Sec.~\ref{sec:optim})\end{tabular}} & \textbf{radam} & & & \textbf{} & \textbf{} & \textbf{} \\ 
\cline{2-7} & \textbf{cadam} & \textbf{\checkmark}  & \textbf{\checkmark} & \textbf{\checkmark} & \textbf{\checkmark} & \textbf{\checkmark} \\ \hline
\end{tabular}

\end{table}
\end{landscape}

\section{Experiment Procedure}\label{sec:app_eval}
The experimental study is carried out in a 3-step procedure. First, we compare the above-mentioned settings under a 6-layer, 6-attention-head complex-valued BERT model that has a hidden size $d_{model} = 384$ and an intermediate size $d_{hidden} = 1536$. We first implement a baseline model with all default settings and trained on the Complex AdamW optimizer. Then, for each experimented setting, we pre-train the model that replaces the default setting with it in the corresponding component while keeping the remaining components as default. Comparing the performance among different models gives the best setting for each component.

Second, we pre-train the model with per-component best settings (\textbf{CVBERT-best}) and compare it with the default complex-valued BERT setting (\textbf{CVBERT-all-split}) as well as the real-valued BERT (\textbf{BERT-base}), on a common 12-layer, 12-attention-head structure. In order for a fair comparison, we align the parameter numbers of complex and real models. In particular, we set the sizes $d_{model} = 768, d_{hidden} = 3072$ for real BERT, $d_{model} = 768,d_{hidden} = 3072$ for all CVBERT variants except \textbf{CVBERT-base}, which has $d_{model} = 768,d_{hidden} = 1536$ and removed query and output projection matrices.

Finally, we evaluate our quantum-compatible setting \textbf{QBERT-base} by comparing with \textbf{CVBERT-base} and \textbf{BERT-base} on a common 12-layer, 12-attention-head structure. In fine-tuning, we also include end-to-end quantum classification models, including \textbf{QCLS-transformer} and \textbf{QCLS-end2end}.  

All our models are pre-trained on 8 Tesla V100 GPU cards with a 32G graphic memory each. The models in the comparative study are pre-trained at a batch size of 256, and the remaining large models are pre-trained at a batch size of 512. We fix the learning rate to be 1e-5 and set a fixed weight decay factor of 1e-4 for the pre-training step. 

For model evaluation, we plot the pre-train learning curves to determine the optimal settings in the first step. For comparing real, complex-valued and quantum-compatible models, we additionally compute their GLUE scores in the fine-tuning step. For each dataset in the collection, we report results on the development sets after fine-tuning the pre-trained model on the corresponding training data. The fine-tuning setup follow the original BERT paper~\citep{devlin2019bert}.

\section{Results of model comparison}~\label{sec:app_ablation}
We have plotted the learning curves of different settings in~\cref{fig:ablation_embeddings,fig:ablation_activations,fig:ablation_normalizations,fig:ablation_dense_layers,fig:ablation_optimizers,fig:ablation_regularizations,fig:ablation_initializations}, up to a total number of 500000 steps. Each figure contains all include settings of a single component, and their learning curves are plotted in different dot shapes and colors. In what follows, we report and interpret the results for each model component.\\

\noindent \textbf{Embedding.} From Fig.~\ref{fig:ablation_embeddings}, the attempt to explicitly encode position in the phases of a complex-valued embedding scheme leads to a low performance, in either the general form (i.e. \textbf{general-complex-embed}) or the frequency-shared version (i.e. \textbf{rotary-embed}). This result illustrates the empirical inferiority of the wave function formulation~\citep{Wang2020encoding} of word semantics in the language model pre-training context. It requires further investigations to account for the huge performance discrepancy of the model under seq2seq~\citep{Wang2020encoding, su2021roformer} and pre-training contexts.\\

\noindent \textbf{Activation.} As shown in Fig.~\ref{fig:ablation_activations}, passing the real part or modulus to the complex-valued query-key inner products does not lead to prominent increases over split softmax activation, even though they are more theoretically sound. On the other hand, the approach to computing attention scores for graph neural network \textbf{(attn-squaredzrelu)} does not apply in the complex-valued transformer structure. For hidden layers, all ReLU and GeLU variants produce close results, even though \textbf{zReLU} and \textbf{ModGeLU} has relatively low performances. Taking modulus softmax for attention layers (\textbf{attn-modsoftmax}) and split GeLU activations (\textbf{hidden-split-gelu}) yield enhanced performance over the default split activation functions, albeit by a tiny margin.\\

\noindent \textbf{Fully-connected Layer.} We conjecture that taking the real part or modulus of dense output to perform NSP or MLM has little impact to the model capacity, since  the pooling layers before the final dense layers are adequate in adapting to both output patterns. As shown in Fig.~\ref{fig:ablation_dense_layers}, whether to take the real part or modulus of dense outputs has literally no impact to model effectiveness, confirming our conjecture.\\

\noindent \textbf{Weight initialization}. Fig.~\ref{fig:ablation_initializations} shows the learning curves of different initialization strategies. From the figure, initializing the model with different standard deviations has an impact on the speed of convergence, but does not influence the convergence loss value. As for Rayleigh-fashion modulus initializers proposed in~\citep{trabelsi2018deep}, the \textbf{Glorot} mode performs apparently better than the \textbf{He} mode in terms of both convergence rate and converging loss value. Similar to 
\textbf{rayleigh-glorot-init}, unitary initialization of complex weights yields a promising learning curve, converging to identical loss values to the default setting (\textbf{split-init-1e-2}) in a faster speed.\\

\noindent \textbf{Normalization.} As shown in Fig.~\ref{fig:ablation_normalizations}, complex layer normalization has identical performance to split layer normalization, despite the differences in the post-normalization variances. We also examined unit-length normalization in order to shed light on the quantum setting. However, it turns out that unit normalization for all token representations (\textbf{unit-norm}) is simply disastrous to model performance. We then take a trade-off approach by unit normalizing the [CLS] token and applying complex layer normalization to the remaining tokens all throughout the model architecture. This \textbf{mixed-layer-norm} setting performs on par to the above normalizations and has a faster convergence speed. Therefore, it provides the motivation for constructing a quantum-friendly pre-trained language model.\\

\noindent \textbf{Regularization}. Fig.~\ref{fig:ablation_regularizations} shows the learning curves of different regularization strategies and different coefficients $\lambda$. When applying orthogonal regularizations to either attention scores or dense weights on its own, a poor-performed learning curve is produced for any value of $\lambda$.  On the stark contrary, the model performs significant better when both regularizers are present, converging to the same loss as the default setting when $\lambda < 1e-6$. This result indicates that orthogonal regularizations does not benefit a deep pre-trained model, different from the findings in~\citep{zhang-etal-2021-orthogonality}. Furthermore, the two types of orthogonality regularizers are apparently more complementary than reported in~\citep{zhang-etal-2021-orthogonality}, possibly due to a more proper implementation and a better alignment of the two regularization terms. \\

\noindent \textbf{Complex Adam vs. Real Adam}. Fig.~\ref{fig:ablation_optimizers} shows a remarkable performance gap between two learning optimization algorithms in training the same model, suggesting a strong favor of our proposed improved optimizer for complex values. \\

\noindent \textbf{Lessons Learned}. The simplest extension of real-valued BERT to the complex domain is to apply the original operations onto the real and imaginary parts of the complex-valued representations. In an attempt to improve the model on top of this all-split extension in the pre-trained context, we explored different implementations for network layers and training configurations, including a large number of settings that have previously been demonstrated useful for small-scale deep complex networks. The experiment result did not indicate positive influences of the majority of included settings, and the modified AdamW optimizer is the only setting that beats the real-valued implementations by a large margin. \\

\noindent \textbf{Best model setting}. In the per-component comparison, the best settings are \textbf{split-embed} for embedding, \textbf{mod-softmax} and \textbf{split-gelu} for attention activations and hidden unit activations respectively, complex layer normalization (\textbf{complex-layer-norm}), and taking the output modulus for computing NSP and MLM losses (\textbf{nsp-modulus} and \textbf{mlm-modulus}). The model is best trained in complex-valued AdamW (\textbf{cadam}) optimizer with no additional orthogonal regularizations applied to dense weights or attention scores. The weights for dense layers and embeddings are best initialized with a normal distribution at a zero mean and 0.01 standard deviation for the real and complex parts, respectively. 

We acknowledge that the per-component comparison is not a perfect way to obtain the best-performed model, since settings on different components are often correlated. For instance, the split embeddings are in favor of the split activation functions and initialization strategies, while the general complex embeddings should be amenable to complex layer normalizations and modulus activation functions.

\begin{figure}[!ht] 
\centering 
\includegraphics[width=0.8\textwidth]{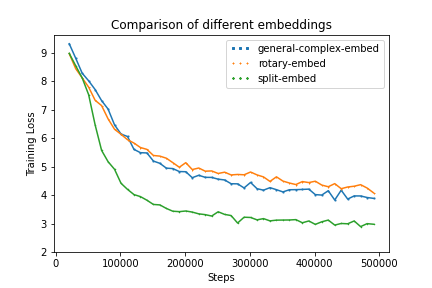}
\caption{Learning curves of different embeddings.}
\label{fig:ablation_embeddings}
\end{figure}

\begin{figure}[!ht] 
\centering 
\includegraphics[width=0.8\textwidth]{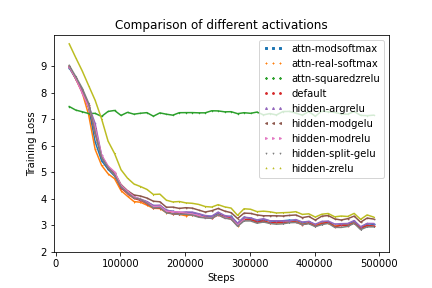}
\caption{Learning curves of different activation functions.}
\label{fig:ablation_activations}

\end{figure}

\begin{figure}[!ht] 
\centering 
\includegraphics[width=0.8\textwidth]{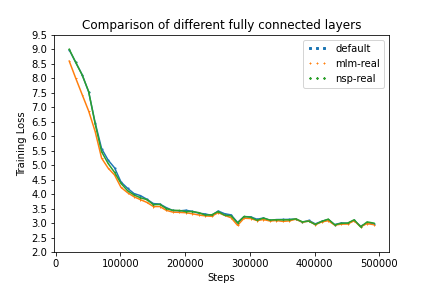}
\caption{Learning curves of different fully-connected layers.}
\label{fig:ablation_dense_layers}

\end{figure}

\begin{figure}[!ht] 
\centering 
\includegraphics[width=0.8\textwidth]{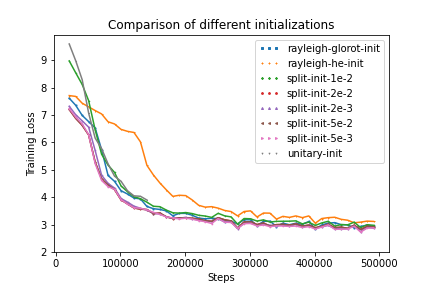}
\caption{Learning curves of different initialization strategies.}
\label{fig:ablation_initializations}

\end{figure}

\begin{figure}[!ht] 
\centering 
\includegraphics[width=0.8\textwidth]{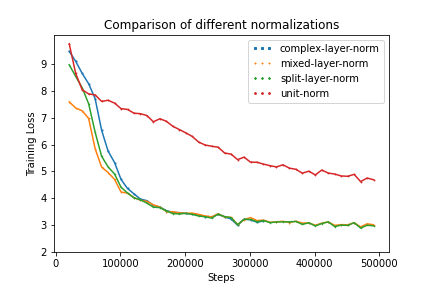}
\caption{Learning curves of different normalizations.}
\label{fig:ablation_normalizations}

\end{figure}

\begin{figure}[!ht] 
\centering 
\includegraphics[width=0.8\textwidth]{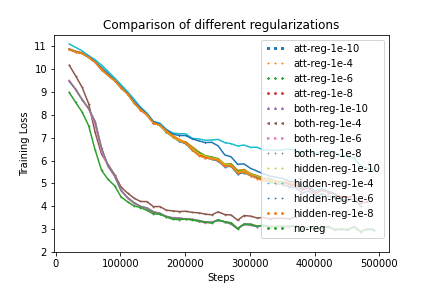}
\caption{Learning curves of different regularization strategies.}
\label{fig:ablation_regularizations}

\end{figure}

\begin{figure}[!ht] 
\centering 
\includegraphics[width=0.8\textwidth]{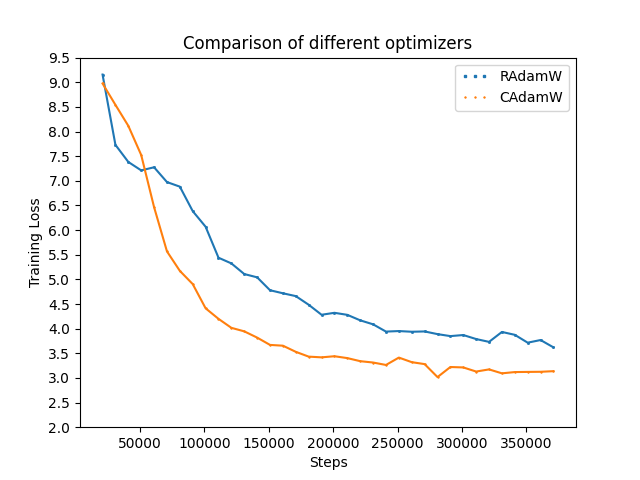}
\caption{Learning curves of using real-valued and complex-valued Adam optimizers to train the same complex-valued model.}
\label{fig:ablation_optimizers}
\end{figure}
